# Supplementary material for: Tectonics on early Earth driven by Earth's changing shape during tidal recession of the Moon
Source: arXiv:2609.22474 source file (2026-09-18)
Supplement: Supplementary file 1 [file SOM.tex]

%%%%%%%%%%%%%%%%%%%%%%%%%%%%%%%%%%%%%%%%%%%%%%%%%%%%%%%%%%%%%%%%%%%%%%%%%%%%
% AGUtmpl.tex: this template file is for articles formatted with LaTeX2e,
% Modified December 2018
%
% This template includes commands and instructions
% given in the order necessary to produce a final output that will
% satisfy AGU requirements.
%
% FOR FIGURES, DO NOT USE \psfrag
%
%%%%%%%%%%%%%%%%%%%%%%%%%%%%%%%%%%%%%%%%%%%%%%%%%%%%%%%%%%%%%%%%%%%%%%%%%%%%
%
% IMPORTANT NOTE:
%
% SUPPORTING INFORMATION DOCUMENTATION IS NOT COPYEDITED BEFORE PUBLICATION.
%
%
%
%%%%%%%%%%%%%%%%%%%%%%%%%%%%%%%%%%%%%%%%%%%%%%%%%%%%%%%%%%%%%%%%%%%%%%%%%%%%
%
% Step 1: Set the \documentclass
%
%
% PLEASE USE THE DRAFT OPTION TO SUBMIT YOUR PAPERS.
% The draft option produces double spaced output.
%
% Choose the journal abbreviation for the journal you are
% submitting to:

% jgrga JOURNAL OF GEOPHYSICAL RESEARCH (use for all of them)
% gbc   GLOBAL BIOCHEMICAL CYCLES
% grl   GEOPHYSICAL RESEARCH LETTERS
% pal   PALEOCEANOGRAPHY
% ras   RADIO SCIENCE
% rog   REVIEWS OF GEOPHYSICS
% tec   TECTONICS
% wrr   WATER RESOURCES RESEARCH
% gc    GEOCHEMISTRY, GEOPHYSICS, GEOSYSTEMS
% sw    SPACE WEATHER
% ms    JAMES
% ef    EARTH'S FUTURE
%
%
%
% (If you are submitting to a journal other than jgrga,
% substitute the initials of the journal for "jgrga" below.)

\documentclass[draft,jgrga]{agutexSI2019}

%fix for infinite shrinkage - thank you internet
\makeatletter
\def\@makecol{\setbox\@outputbox
     \vbox{\boxmaxdepth \maxdepth
\ifdim\ht\dbltopins<1pt\else\unvbox\dbltopins\fi
     \unvbox\@cclv
\ifdim\ht\dblbotins<1pt\else\unvbox\dblbotins\fi%
\ifvoid\footins\else\vskip\skip\footins\footnoterule\unvbox\footins\fi
%\vss
\vskip 0pt plus 1fil minus \maxdimen
}%
%\global\savefigandtabnumber\figandtabnumber
%\global\advance\savefigandtabnumber by 1 %% Because loop stops one short
                                         %% of the total number of figs
\global\savedblfigandtabnumber\dblfigandtabnumber
   \xdef\@freelist{\@freelist\@midlist}\gdef\@midlist{}\@combinefloats
   \setbox\@outputbox\vbox to\@colht{\boxmaxdepth\maxdepth
   \@texttop\dimen128=\dp\@outputbox\unvbox\@outputbox
   \vskip-\dimen128\@textbottom}%
   \global\maxdepth\@maxdepth}
\makeatother

%%%%%%%%%%%%%%%%%%%%%%%%%%%%%%%%%%%%%%%%%%%%%%%%%%%%%%%%%%%%%%%%%%%%%%%%%
%
%  SUPPORTING INFORMATION TEMPLATE
%
%% ------------------------------------------------------------------------ %%
%
%
%Please use this template when formatting and submitting your Supporting Information.

%This template serves as both a “table of contents” for the supporting information for your article and as a summary of files.
%
%
%OVERVIEW
%
%Please note that all supporting information will be peer reviewed with your manuscript. It will not be copyedited if the paper is accepted.
%In general, the purpose of the supporting information is to enable authors to provide and archive auxiliary information such as data tables, method information, figures, video, or computer software, in digital formats so that other scientists can use it.
%The key criteria are that the data:
% 1. supplement the main scientific conclusions of the paper but are not essential to the conclusions (with the exception of
%    including %data so the experiment can be reproducible);
% 2. are likely to be usable or used by other scientists working in the field;
% 3. are described with sufficient precision that other scientists can understand them, and
% 4. are not exe files.
%
%USING THIS TEMPLATE
%
%***All references should be included in the reference list of the main paper so that they can be indexed, linked, and counted as citations.  The reference section does not count toward length limits.
%
%All Supporting text and figures should be included in this document. Insert supporting information content into each appropriate section of the template. To add additional captions, simply copy and paste each sample as needed.

%Tables may be included, but can also be uploaded separately, especially if they are larger than 1 page, or if necessary for retaining table formatting. Data sets, large tables, movie files, and audio files should be uploaded separately. Include their captions in this document and list the file name with the caption. You will be prompted to upload these files on the Upload Files tab during the submission process, using file type “Supporting Information (SI)”

%IMPORTANT NOTE ON FIGURES AND TABLES
% Placeholders for figures and tables appear after the \end{article} command, after references.
% DO NOT USE \psfrag or \subfigure commands.
%
 \usepackage{graphicx}
%
%  Uncomment the following command to allow illustrations to print
%   when using Draft:
 \setkeys{Gin}{draft=false}
%
% You may need to use one of these options for graphicx depending on the driver program you are using. 
%
% [xdvi], [dvipdf], [dvipsone], [dviwindo], [emtex], [dviwin],
% [pctexps],  [pctexwin],  [pctexhp],  [pctex32], [truetex], [tcidvi],
% [oztex], [textures]
%
%
%% ------------------------------------------------------------------------ %%
%
%  ENTER PREAMBLE
%
%% ------------------------------------------------------------------------ %%

% Author names in capital letters:
\authorrunninghead{LOCK}

% Shorter version of title entered in capital letters:
\titlerunninghead{TECTONICS ON EARLY EARTH}

%Corresponding author mailing address and e-mail address:
%\authoraddr{Corresponding author: A. B. Smith,
%Department of Hydrology and Water Resources, University of
%Arizona, Harshbarger Building 11, Tucson, AZ 85721, USA.
%(a.b.smith@hwr.arizona.edu)}

%reference things in the main text
\usepackage{xr}
\externaldocument{main}

\begin{document}

%% ------------------------------------------------------------------------ %%
%
%  TITLE
%
%% ------------------------------------------------------------------------ %%

%\includegraphics{agu_pubart-white_reduced.eps}


\title{Supporting Information for "Tectonics on early Earth driven by Earth's changing shape during tidal recession of the Moon"}
%
% e.g., \title{Supporting Information for "Terrestrial ring current:
% Origin, formation, and decay $\alpha\beta\Gamma\Delta$"}
%
%DOI: 10.1002/%insert paper number here%

%% ------------------------------------------------------------------------ %%
%
%  AUTHORS AND AFFILIATIONS
%
%% ------------------------------------------------------------------------ %%


% List authors by first name or initial followed by last name and
% separated by commas. Use \affil{} to number affiliations, and
% \thanks{} for author notes.
% Additional author notes should be indicated with \thanks{} (for
% example, for current addresses).

% Example: \authors{A. B. Author\affil{1}\thanks{Current address, Antartica}, B. C. Author\affil{2,3}, and D. E.
% Author\affil{3,4}\thanks{Also funded by Monsanto.}}

\authors{S. J. Lock\affil{1,2}}


% \affiliation{1}{First Affiliation}
% \affiliation{2}{Second Affiliation}
% \affiliation{3}{Third Affiliation}
% \affiliation{4}{Fourth Affiliation}
\affiliation{1}{School of Earth Sciences, University of Bristol, Bristol, BS8 1RJ, UK}
\affiliation{2}{Formerly: Division of Geological and Planetary Sciences, California Institute of Technology, Pasadena, CA 91125, USA}

% \correspondingauthor{S. J. Lock}{s.lock@bristol.ac.uk}


%% ------------------------------------------------------------------------ %%
%
%  BEGIN ARTICLE
%
%% ------------------------------------------------------------------------ %%

% The body of the article must start with a \begin{article} command
%
% \end{article} must follow the references section, before the figures
%  and tables.
\begin{article}

%% ------------------------------------------------------------------------ %%
%
%  TEXT
%
%% ------------------------------------------------------------------------ %%



\noindent\textbf{Contents of this file}
%%%Remove or add items as needed%%%
\begin{enumerate}
\item Figures S1 to S4
\item Captions for Movies S1 to S6
%if Tables are larger than 1 page, upload as separate excel file
\end{enumerate}
\noindent\textbf{Additional Supporting Information (Files uploaded separately)}
\begin{enumerate}
\item Movies S1 to S6. Supplementary movie files can be found at: {\small {\tt tinyurl.com/2ucc3uex}}
\item Scripts to reproduce results presented in the manuscript. Location TBD
\end{enumerate}


%%%%%%%%%%%%%%%%%%%%%%%%%%%%%%%%%%%%%%%%%%%%%%%%%%%%%%%%%%%%%%%%%%%%%%%%%
\bibliography{References_processed}

% \section*{Supplementary Figures}
\end{article}
% \clearpage

\begin{figure}
\centering
\noindent\includegraphics[scale=0.93]{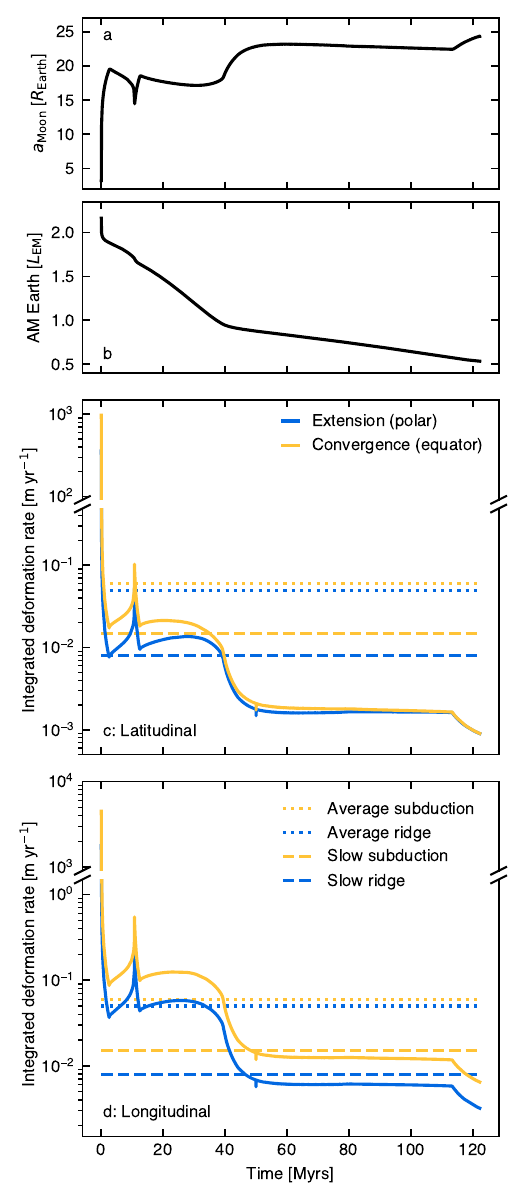}
\caption{Caption on next page.}
\end{figure}
\addtocounter{figure}{-1}
\begin{figure}
\centering
\caption{Different tidal evolution scenarios can lead to very different crustal deformation histories. Presented is the time dependent crustal deformation for the tidal evolution scenario shown in Figure~3 of \citeA{Cuk2021} where Earth initially has a large obliquity causing angular momentum to be transferred away from the Earth-Moon system during the Laplace plane transition. In this particular example, the Earth-Moon system has a total initial angular momentum of 2.37~$L_{\rm EM}$ and Earth begins with an obliquity of 65$^{\circ}$. The tidal properties of the Earth and Moon were constant with $k_{2,{\rm Earth}}/Q_{\rm Earth}=k_{2,{\rm Moon}}/Q_{\rm Moon}=1\times10^{-2}$. Panels, lines and colors are the same as those in Figure~\ref{fig:canonical_PTcomp}. Note that, unlike in Figure~\ref{fig:canonical_PTcomp}, the time axis is linear rather than logarithmic. Movie~\ref{sup:movie:Cuk_example2} contains an animated version of elements of this figure showing the change in shape and deformation rate during lunar tidal evolution.
}
\label{sup:fig:CukFig3_PTcomp}
\end{figure}

\begin{figure}
\centering
\includegraphics[scale=0.93]{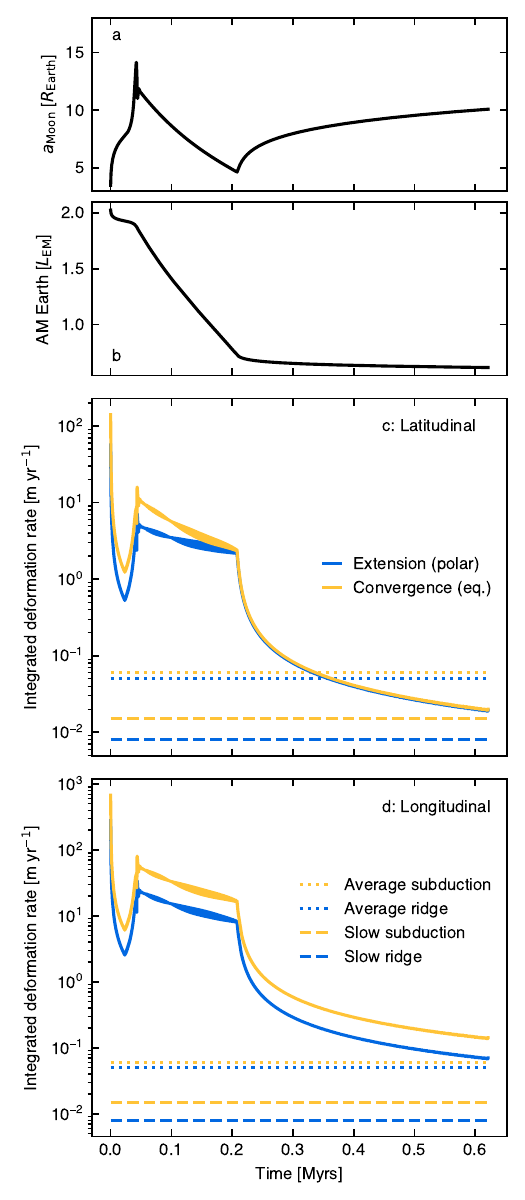}
\caption{Caption on next page.}
\end{figure}
\addtocounter{figure}{-1}
\begin{figure}
\centering
\caption{
The rate of surface deformation in high-angular momentum scenarios is highly dependent on the tidal parameters of the Earth and Moon. Presented are the maximum integrated surface deformation rates as a function of time in a scenario in which angular momentum is transferred away from the Earth-Moon system when the system is captured in a limit cycle associated with the evection resonance \cite{Rufu2020}. In this specific scenario, the tidal $A$ parameter was set at 5 and the tidal time constant $t_T=4.9\times 10^6$~s, an effective $k_{2,{\rm Earth}}/Q_{\rm Earth}=2.4 \times 10^{-3}$ ($Q_{\rm Earth}/k_{2,{\rm Earth}}=410$). This scenario is labelled as example 1 in Figure~\ref{fig:Rufu_comparison}. Examples with different fixed tidal parameters are shown in Figures~\ref{sup:fig:RufuA500_PTcomp} and \ref{sup:fig:RufuA10k_PTcomp}. Panels, lines and colors are the same as those in Figure~\ref{fig:canonical_PTcomp}. Note that, unlike in Figure~\ref{fig:canonical_PTcomp}, the time axis is linear rather than logarithmic. Movie~\ref{sup:movie:RufuA5} contains an animated version of elements of this figure showing the change in shape and deformation rate during lunar tidal evolution.
}
\label{sup:fig:RufuA5_PTcomp}
\end{figure}



\begin{figure}
\centering
\includegraphics[scale=0.93]{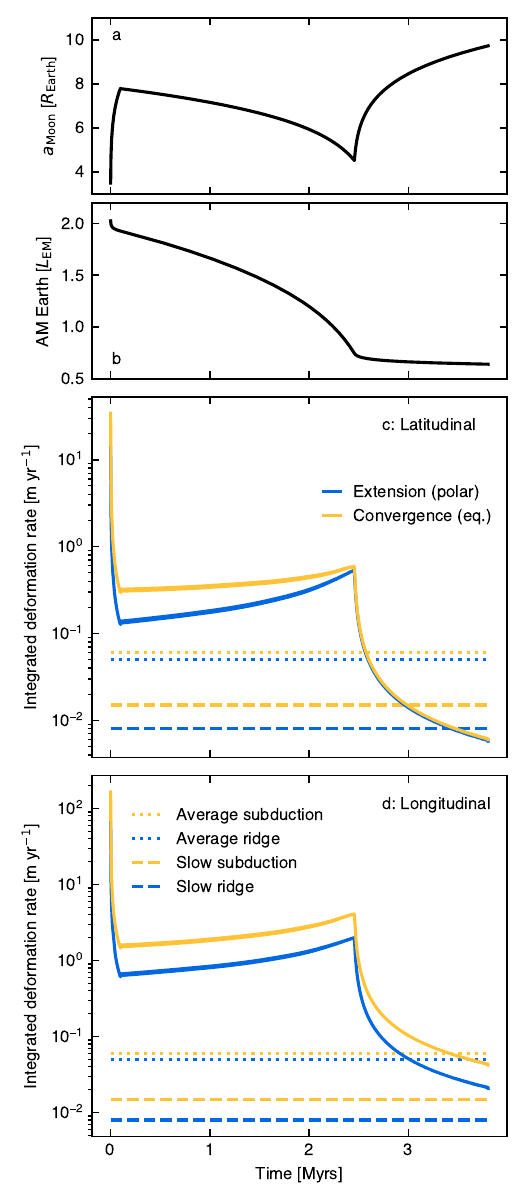}
\caption{As Figure~\ref{sup:fig:RufuA5_PTcomp} but for a calculation with $A=500$ and $t_{T}=2.0\times 10^7$~s, an effective $k_{2,{\rm Earth}}/Q_{\rm Earth}=5.9 \times 10^{-4}$ ($Q_{\rm Earth}/k_{2,{\rm Earth}}=1.7\times 10^3$). This scenario is labelled as example 2 in Figure~\ref{fig:Rufu_comparison}. Movie~\ref{sup:movie:RufuA500} contains an animated version of elements of this figure showing the change in shape and deformation rate during lunar tidal evolution.}
\label{sup:fig:RufuA500_PTcomp}
\end{figure}


\begin{figure}
\centering
\includegraphics[scale=0.93]{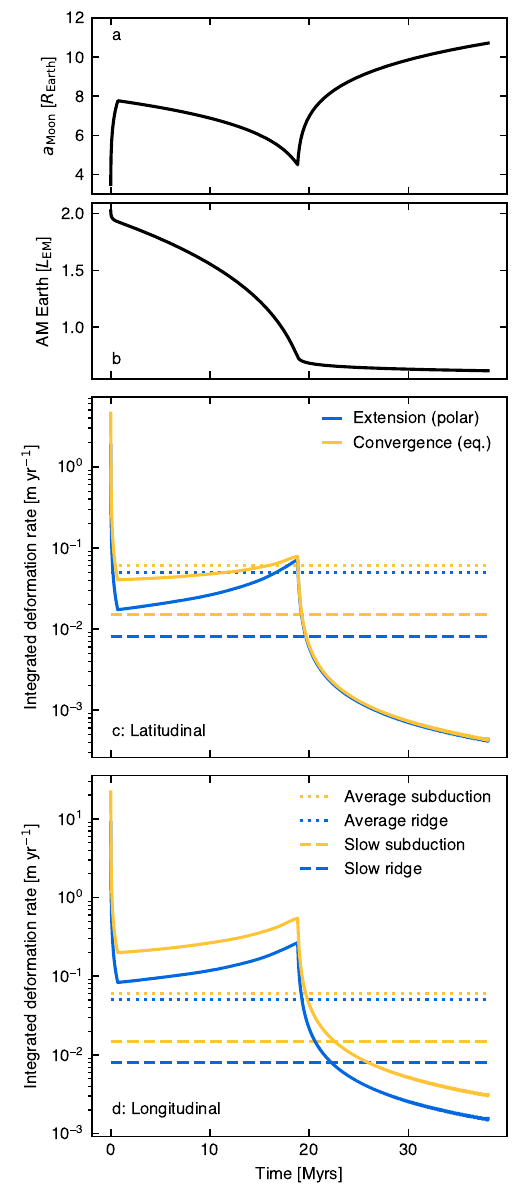}
\caption{As Figure~\ref{sup:fig:RufuA5_PTcomp} but for a calculation with $A=10^4$ and $t_{T}=1.5\times 10^8$~s, an effective $k_{2,{\rm Earth}}/Q_{\rm Earth}=8.3 \times 10^{-5}$ ($Q_{\rm Earth}/k_{2,{\rm Earth}}=1.2\times 10^4$). This scenario is labelled as example 3 in Figure~\ref{fig:Rufu_comparison}. Movie~\ref{sup:movie:RufuA10k} contains an animated version of elements of this figure showing the change in shape and deformation rate during lunar tidal evolution.}
\label{sup:fig:RufuA10k_PTcomp}
\end{figure}







%%%%%%%%%%%%%%%%%%%%%%%%%%%%%%%%%%%%%%%%%%%%%%%%%%%%%%%%%%%%%%%%%
%%%%%%%%%%%%%%%%%%%%%%%%%%%%%%%%%%%%%%%%%%%%%%%%%%%%%%%%%%%%%%%%%
\renewcommand{\figurename}{Movie}
\setcounter{figure}{0}


\begin{figure}
\centering
\caption{Animated version of elements of Figures~\ref{fig:canonical_PTcomp} and \ref{sup:fig:canonical_example}. Shown are the lunar semi-major axis (A), angular momentum of Earth (B), maximum integrated convergence (yellow) and extension (blue) rates in the longitudinal direction (C), and rate of change of local length in the longitudinal direction (D) as a function of time for a simple canonical tidal evolution model in which the angular momentum of the Earth-Moon system remains constant (for details see Section~\ref{sup:sec:tidal_model}).  In this example, the Moon is assumed to have formed at the Roche limit ($2.9$~$R_{\rm Earth}$), and the tidal Love number ($k_{2,{\rm Earth}}$) and tidal quality factor ($Q_{\rm Earth}$) of Earth were constant and set to those of the present-day solid Earth, 0.3 and 100 respectively \cite{Yoder1995,Ray2012}. Panel D shows the shape of Earth at a given time to scale with crustal deformations projected onto the surface as if seen by a distant observer in the equator. In D, the horizontal black solid lines shows the latitude of zero deformation and the black dashed line is the initial shape of the planet.}
\label{sup:movie:canonical_example}
\end{figure}

\begin{figure}
\centering
\caption{Animated version of elements of Figures~\ref{fig:CukFig7_PTcomp} and \ref{sup:fig:Cuk_example} showing the time dependent crustal deformation for the tidal evolution scenario presented in Figure~7 of \citeA{Cuk2021} where Earth initially has a large initial obliquity causing angular momentum to be transferred away from the Earth-Moon system during the Laplace plane transition. Panels and lines are the same as in Movie~\ref{sup:movie:canonical_example}.}
\label{sup:movie:Cuk_example}
\end{figure}

\begin{figure}
\centering
\caption{Animated version of elements of Figure~\ref{sup:fig:CukFig3_PTcomp} showing the time dependent crustal deformation for the tidal evolution scenario presented in Figure~3 of \citeA{Cuk2021} where Earth initially has a large initial obliquity causing angular momentum to be transferred away from the Earth-Moon system during the Laplace plane transition.  Panels and lines are the same as in Movie~\ref{sup:movie:canonical_example}.}
\label{sup:movie:Cuk_example2}
\end{figure}

\begin{figure}
\centering
\caption{Animated version of elements of Figure~\ref{sup:fig:RufuA5_PTcomp} showing the time dependent crustal deformation in a scenario in which angular momentum is transferred away from the Earth-Moon system when the system is captured in a limit cycle associated with the evection resonance \cite{Rufu2020}. In this specific example, the tidal $A$ parameter was set at 5 and the tidal time constant $t_T=4.9\times 10^6$, an effective $k_{2,{\rm Earth}}/Q_{\rm Earth}=2.4 \times 10^{-3}$ ($Q_{\rm Earth}/k_{2,{\rm Earth}}=410$). Panels and lines are the same as in Movie~\ref{sup:movie:canonical_example}.}
\label{sup:movie:RufuA5}
\end{figure}

\begin{figure}
\centering
\caption{Animated version of elements of Figure~\ref{sup:fig:RufuA500_PTcomp} showing the time dependent crustal deformation in a scenario in which angular momentum is transferred away from the Earth-Moon system when the system is captured in a limit cycle associated with the evection resonance \cite{Rufu2020}. In this specific example, $A=500$ and $t_{T}=2.0\times 10^7$~s, an effective $k_{2,{\rm Earth}}/Q_{\rm Earth}=5.9 \times 10^{-4}$ ($Q_{\rm Earth}/k_{2,{\rm Earth}}=1.7\times 10^3$). Panels and lines are the same as in Movie~\ref{sup:movie:canonical_example}.}
\label{sup:movie:RufuA500}
\end{figure}

% \clearpage
% 

\begin{figure}
\centering
\caption{Animated version of elements of Figure~\ref{sup:fig:RufuA10k_PTcomp} showing the time dependent crustal deformation in a scenario in which angular momentum is transferred away from the Earth-Moon system when the system is captured in a limit cycle associated with the evection resonance \cite{Rufu2020}. In this specific example, $A=10^4$ and $t_{T}=1.5\times 10^8$~s, an effective $k_{2,{\rm Earth}}/Q_{\rm Earth}=8.3 \times 10^{-5}$ ($Q_{\rm Earth}/k_{2,{\rm Earth}}=1.2\times 10^4$). Panels and lines are the same as in Movie~\ref{sup:movie:canonical_example}.}
\label{sup:movie:RufuA10k}
\end{figure}

% \vspace{100pt}
% \clearpage
% \vspace{100pt}
\end{document}
